# Supplementary material for: Particle-based, rapid incremental smoother meets particle Gibbs
Source: arXiv:2209.10351 source file (2022-09-21)
Supplement: Supplementary file 1 [file numerics_appendix.tex]

%For the LGSS model, the values of the parameters ($A,Q,B,R$) are ($0.46, 0.15, 0.6, 0.06$).
